# Supplementary material for: On denoising modulo 1 samples of a function
Source: arXiv:1710.10210 source file (2018-04-02)
Supplement: Supplementary file 1 [file appendix_noise.tex]

%---------------------------------------------------
% Appendix containing proofs for random noise model
%---------------------------------------------------
%
%-----------------------------------
% Useful concentration inequalities
%-----------------------------------
\section{Useful concentration inequalities} \label{sec:app_conc_ineq}
We present in this section some useful concentration inequalities, that will be employed 
as a tool to prove our other results. Recall that for a random variable $X$, its sub-Gaussian norm 
$\norm{X}_{\psi_2}$ is defined as 
\begin{equation}
\norm{X}_{\psi_2} := \sup_{p \geq 1} \frac{(\expec \abs{X}^p)^{1/p}}{\sqrt{p}}.
\end{equation}
Moreover, $X$ is a sub-Gaussian random variable if $\norm{X}_{\psi_2}$ is finite. 
For instance, consider a bounded random variable $X$ with $\abs{X} \leq M$. Then, $X$ 
is a sub-Gaussian random variable with $\norm{X}_{\psi_2} \leq M$ \cite[Example 5.8]{vershynin2012}.

We begin with the well known 
Hanson Wright inequality \cite{Hanson71} for concentration of random quadratic forms. 
The following version is taken from \cite{rudelson2013}.
%
%----------------------------
% Hanson Wright inequality
%----------------------------
\begin{theorem}[\cite{rudelson2013}] \label{thm:hanson_wright} 
Let $(X_1 \ X_2 \ \cdots \ X_n) \in \matR^{n}$ be a random vector with independent components $X_i$ 
satisfying $\expec[X_i] = 0$ and $\norm{X_i}_{\psi_2} \leq K$. Let $\matA$ be a $n \times n$ matrix. 
Then for every $t \geq 0$
\begin{equation}
\mathbb{P}(\abs{X^T \matA X - \expec[X^T \matA X]} \geq t) \leq 
2\exp\left( -c \min \left(\frac{t^2}{K^4\norm{\matA}_F^2} , \frac{t}{K^2\norm{\matA}}\right)  \right)
\end{equation}
for an absolute constant $c > 0$.
\end{theorem}
Next, we recall the following Hoeffding type inequality for sums of independent sub-Gaussian random variables.
%
%-------------------------------------------
% Hoeffding type concentration inequality
%--------------------------------------------
\begin{proposition} \cite[Proposition 5.10]{vershynin2012} \label{prop:hoeff_subgauss_conc}
Let $X_1,\dots,X_n$ be independent  centered sub-Gaussian random variables and let $K = \max_i \norm{X_i}_{\psi_2}$. 
Then for every $\veca \in \matR^n$, and every $t \geq 0$, we have
\begin{equation}
\prob(\abs{\sum_{i=1}^n a_i X_i} \geq t) \leq e \cdot \exp\left(-\frac{c^{\prime} t^2}{K^2 \norm{\veca}_2^2}\right).
\end{equation}
where $c^{\prime} > 0$ is an absolute constant.
\end{proposition}

%--------------------------------------------------------------------------------
% Proof of Proposition for concentration results: Bernoulli uniform noise model
%--------------------------------------------------------------------------------
\section{Proof of Proposition \ref{prop:bern_unif_conc}} \label{sec:proof_prop_bern_unif}
Let us first recall the definition of $\veczbar$ from \eqref{eq:real_notat}. For clarity of notation, 
we will denote $\veczbar_R = \real(\vecz) \in \matR^n$ and $\veczbar_I = \imag(\vecz) \in \matR^n$, so  
$\veczbar = [\veczbar_R^T \quad \veczbar_I^T]^T \in \matR^{2n}$. Clearly, $(z_i)_{i=1}^n$ are 
independent, complex valued random variables. Note that 
\begin{equation}
(\veczbar_R)_i = \cos(2\pi y_i) = \left\{
\begin{array}{rl}
\cos(2\pi (f_i\bmod 1)) \quad ; & \text{if} \ \eta_i = 0 \\
\cos(2\pi u_i) \quad ; & \text{if} \ \eta_i = 1
\end{array} \right. \quad ; \quad i=1,\dots,n.
\end{equation}
and 
\begin{equation}
(\veczbar_I)_i = \sin(2\pi y_i) = \left\{
\begin{array}{rl}
\sin(2\pi (f_i\bmod 1)) \quad ; & \text{if} \ \eta_i = 0 \\
\sin(2\pi u_i) \quad ; & \text{if} \ \eta_i = 1
\end{array} \right. \quad ; \quad i=1,\dots,n.
\end{equation}
Since $(\eta_i)_{i=1}^{n}$ and $(u_i)_{i=1}^{n}$ are i.i.d random variables, hence the components of $\veczbar_R$ are independent 
real valued random variables. The same is true for the components of $\veczbar_I$.
\begin{enumerate}
%-----------------------------------
% Lower bounding the quadratic term
%-----------------------------------
\item \underline{\textbf{Lower bounding $\frac{1}{2n} \veczbar^T \Hbar \veczbar$}} 

To begin with, note that $\veczbar^T \Hbar \veczbar = \veczbar_R^T (\lambda L) \veczbar_R + \veczbar_I^T (\lambda L) \veczbar_I$. 
Denote $\mean_R = \expec[\veczbar_R] \in \matR^n$, and $\mean_I = \expec[\veczbar_I] \in \matR^n$. 
We see that 
\begin{align}
(\mean_R)_i &= \expec[(\veczbar_R)_i] \\
&= (1-p)\cos(2\pi (f_i\bmod 1)) + p\expec[\cos(2\pi u_i)] \\
&= (1-p)\cos(2\pi (f_i\bmod 1))
\end{align}
since $\expec[\cos(2\pi u_i)] = 0$ for $i=1,\dots,n$. 
Similarly, $(\mean_I)_i = (1-p)\sin(2\pi (f_i\bmod 1))$. Hence, 
%--------------------
\begin{equation} \label{eq:bern_unif_temp0}
\mean_R = (1-p) \real(\vechtil) \quad \text{and} \quad \mean_I = (1-p) \imag(\vechtil)
\end{equation}
%--------------------
We now focus on lower bounding the term $\veczbar_R^T L \veczbar_R$. Clearly, 
%------------------------
\begin{align}
\veczbar_R^T L \veczbar_R
&= (\veczbar_R - \mean_R + \mean_R)^T L (\veczbar_R - \mean_R + \mean_R) \\
&= (\veczbar_R - \mean_R)^T L (\veczbar_R - \mean_R) + 2(\veczbar_R - \mean_R)^T L \mean_R + \mean_R^T L \mean_R. \label{eq:bern_unif_temp1}
\end{align}
%------------------------
%
The first two terms in \eqref{eq:bern_unif_temp1} are random; we now proceed to lower bound them w.h.p starting with the first term. 
Let us note that 
\begin{align}
\expec[(\veczbar_R - \mean_R)^T L (\veczbar_R - \mean_R)] 
&= \sum_{i=1}^n \expec[(\veczbar_R)_i - (\mean_R)_i]^2 L_{ii} \nonumber \\
		&+  \sum_{i \neq j} \underbrace{\expec[((\veczbar_R)_i - (\mean_R)_i)((\veczbar_R)_j - (\mean_R)_j)]}_{ = 0} L_{ij} \label{eq:bern_unif_tempA} \\
&= \sum_{i=1}^n (\expec[(\veczbar_R)_i]^2 - (\mean_R)_i^2) \deg(i) \label{eq:bern_unif_temp2}
\end{align}
since the cross terms in \eqref{eq:bern_unif_tempA} are zero. Some simple calculation reveals that
%---------------
\begin{align}
\expec[(\veczbar_R)_i]^2 &= \frac{1}{2} + \frac{1}{2}(1-p) \cos(4\pi(f_i\bmod 1)) \label{eq:bern_unif_temp3} \\
\text{and} \quad (\mean_R)_i^2 &= \frac{(1-p)^2}{2} + \frac{(1-p)^2}{2} \cos(4\pi(f_i \bmod 1)). \label{eq:bern_unif_temp4}
\end{align}
%---------------
for $i=1,\dots,n$. Plugging \eqref{eq:bern_unif_temp3}, \eqref{eq:bern_unif_temp4} in \eqref{eq:bern_unif_temp2}, and 
observing that $k \leq \deg(i) \leq 2k$, one can easily verify that 
\begin{align}
\frac{pnk}{2} \leq \expec[(\veczbar_R - \mean_R)^T L (\veczbar_R - \mean_R)] \leq \frac{3pnk}{2}.  \label{eq:bern_unif_temp5}
\end{align}
Now for each $i = 1,\dots,n$, the random variables $(\veczbar_R)_i - (\mean_R)_i$ are zero mean, and are also uniformly bounded 
as 
\begin{align}
\abs{(\veczbar)_i - (\mean_R)_i} = \abs{\cos(2\pi y_i) - (1-p)\cos(2\pi(f_i \bmod 1))} \leq 2.
\end{align}
Hence $\norm{(\veczbar)_i - (\mean_R)_i}_{\psi_2} \leq 2$ for each $i$. Therefore, applying Hanson Wright inequality to 
$(\veczbar_R - \mean_R)^T L (\veczbar_R - \mean_R)$ yields
%
%---------------
\begin{align}
\prob(\abs{(\veczbar_R - \mean_R)^T L (\veczbar_R - \mean_R) - \expec[(\veczbar_R - \mean_R)^T L (\veczbar_R - \mean_R)]} \geq t) \nonumber \\
\leq 2\exp\left( -c \min \left(\frac{t^2}{16\norm{L}_F^2}, \frac{t}{4\norm{L}}\right) \right). \label{eq:bern_unif_temp6}
\end{align}
%---------------
Since $\deg(i) \leq 2k$ for each $i=1,\dots,n$, therefore Gershgorins disk theorem yields the estimate $\norm{L} \leq 4k$. 
Moreover, $\norm{L}_F^2 \leq \sum_i ((2k)^2 + 2k) \leq 8k^2n$. Plugging $t = \frac{\varepsilon p n k}{2}$ for $\varepsilon \in (0,1)$, 
we observe that
\begin{align} 
\frac{t^2}{16\norm{L}_F^2} &\geq \frac{(\varepsilon^2 p^2 n^2 k^2)/4}{128 k^2 n} = \frac{\varepsilon^2 p^2 n}{512}, \\
\text{and} \quad \frac{t}{4\norm{L}} &\geq \frac{(\varepsilon p n k)/2}{16 k} = \frac{\varepsilon p n}{32}. 
\end{align}
Thus, $\min\set{\frac{t^2}{16\norm{L}_F^2}, \frac{t}{4\norm{L}}} \geq \frac{\varepsilon^2 p^2 n}{512}$. Plugging this estimate 
in \eqref{eq:bern_unif_temp6} for the aforementioned choice of $t$, and using the bounds in \eqref{eq:bern_unif_temp5}, 
we have with probability at least $1 - 2\exp\left(-\frac{c \varepsilon^2 p^2 n}{512}\right)$ that
%
%-------------------
\begin{align}
\frac{pnk}{2}(1-\varepsilon) \leq (\veczbar_R - \mean_R)^T L (\veczbar_R - \mean_R) \leq pnk\left(3 + \frac{\varepsilon}{2}\right). \label{eq:bern_unif_temp7}
\end{align}
%------------------
We now turn our attention to the second term in \eqref{eq:bern_unif_temp1} namely $2(\veczbar_R - \mean_R)^T L \mean_R$.
Recall that $(\veczbar_R)_i - (\mean_R)_i$ are independent, zero mean sub-Gaussian random variables with $\norm{(\veczbar_R)_i - (\mean_R)_i}_{\psi_2} \leq 2$, 
for each $i$. Hence invoking Proposition \ref{prop:hoeff_subgauss_conc} gives us
\begin{align}
\prob(\abs{\dotprod{\veczbar_R - \mean_R}{2 L \mean_R}} \geq t) 
&\leq e\cdot \exp\left(-\frac{c^{\prime} t^2}{4 \norm{2 L \mean_R}_2^2}\right) \\ 
&\leq e\cdot \exp\left(-\frac{c^{\prime} t^2}{16 \norm{L}^2 \norm{\mean_R}_2^2}\right) \\ 
&\leq e\cdot \exp\left(-\frac{c^{\prime} t^2}{256 k^2 n}\right), \label{eq:bern_unif_temp8}
\end{align}
where in \eqref{eq:bern_unif_temp8}, we used the bounds $\norm{L} \leq 4k$ and $\norm{\mean_R}_2^2 \leq n$.
Plugging $t = \frac{pnk(1-\varepsilon)}{3}$ in \eqref{eq:bern_unif_temp8}, we have that the following 
holds with probability at least $1 - e \cdot \exp\left(-\frac{c^{\prime} p^2 n (1-\varepsilon)^2}{2304}\right)$.
%
%--------------------
\begin{align}
\abs{\dotprod{\veczbar_R - \mean_R}{2 L \mean_R}} \leq \frac{pnk(1-\varepsilon)}{3}. \label{eq:bern_unif_temp9}
\end{align}
%--------------------
Combining \eqref{eq:bern_unif_temp7}, \eqref{eq:bern_unif_temp9} and applying the union bound, we have with 
probability at least $1 - e \cdot\exp\left(-\frac{c^{\prime} p^2 n (1-\varepsilon)^2}{2304}\right) - 2\exp\left(-\frac{c \varepsilon^2 p^2 n}{512}\right)$
that the following bound holds.
\begin{equation} 
\veczbar_R^T L \veczbar_R \geq \frac{pnk}{6}(1-\varepsilon) + \mean_R^T L \mean_R. \label{eq:bern_unif_temp10}
\end{equation}
By proceeding as above, one can verify that with 
probability at least $1 - e \cdot \exp\left(-\frac{c^{\prime} p^2 n (1-\varepsilon)^2}{2304}\right)$ $- 2\exp\left(-\frac{c \varepsilon^2 p^2 n}{512}\right)$, 
the following bound holds.
\begin{equation} 
\veczbar_I^T L \veczbar_I \geq \frac{pnk}{6}(1-\varepsilon) + \mean_I^T L \mean_I. \label{eq:bern_unif_temp11}
\end{equation}
Combining \eqref{eq:bern_unif_temp10}, \eqref{eq:bern_unif_temp11} and applying the union bound, we have 
with probability at least $1 - 2e\cdot\exp\left(-\frac{c^{\prime} p^2 n (1-\varepsilon)^2}{2304}\right) - 4\exp\left(-\frac{c \varepsilon^2 p^2 n}{512}\right)$ 
that 
%
%----------------------
\begin{align}
\frac{1}{2n} \veczbar^T \Hbar \veczbar 
&= \frac{1}{2n} \lambda(\veczbar_R^T L \veczbar_R + \veczbar_I^T L \veczbar_I) \\
&\geq \frac{\lambda p n k}{6n}(1-\varepsilon) + \frac{1}{2n}\left(\mean_R^T (\lambda L) \mean_R + \mean_I^T (\lambda L) \mean_I \right) \label{eq:bern_unif_temp12}  \\
&= \frac{\lambda p k}{6}(1-\varepsilon) + (1-p)^2 \frac{1}{2n} \vechtilbar \Hbar \vechtilbar \label{eq:bern_unif_temp13}
\end{align}
%------------------------
holds. To go from \eqref{eq:bern_unif_temp12} to \eqref{eq:bern_unif_temp13}, we used \eqref{eq:bern_unif_temp0} 
along with the definition of $\Hbar$ (see also Appendix \ref{sec:qcqp_compl_to_real}). 
This completes the derivation of the lower bound on $\frac{1}{2n} \veczbar^T \Hbar \veczbar$.

%
%--------------------------------
% Upper bounding the noise term
%--------------------------------
\item \underline{\textbf{Upper bounding $\norm{\veczbar - \vechtilbar}_2$}}
By recalling the definition of $\veczbar,\vechtilbar \in \matR^{2n}$ from \eqref{eq:real_notat}, we note that
\begin{align}
\norm{\veczbar - \vechtilbar}_2^2 
&= \left|\left|\begin{pmatrix}
  \real(\vecz) \\ \imag(\vecz) 
 \end{pmatrix} 
- \begin{pmatrix}
  \real(\vechtil) \\ \imag(\vechtil) 
 \end{pmatrix}\right|\right|_2^2 \\
&= \norm{\vecz - \vechtil}_2^2 \\
&= 2n - (\vecz^{*}\vechtil + \vechtil^{*}\vecz) \\
&= 2n - \sum_{i=1}^{n}(\exp(\iota 2\pi(f_i\bmod 1 - y_i)) + \exp(-\iota 2\pi(f_i\bmod 1 - y_i))) \\
&= 2n - \sum_{i=1}^{n}\underbrace{(2\cos (2\pi(f_i \bmod 1 - y_i)))}_{M_i}. \label{eq:nois_conc_temp0}
\end{align}
Clearly $(M_i)_{i=1}^{n}$ are independent sub-Gaussian random variables with $\abs{M_i} \leq 2$;  
hence $\norm{M_i}_{\psi_2} \leq 2$ for each $i$. Moreover,
\begin{align}
\expec[M_i] 
&= 2(1-p) + p\expec[(2\cos (2\pi(f_i \bmod 1 - u_i)))] \\
&= 2(1-p) + p\int_{0}^{1} 2\cos (2\pi(f_i \bmod 1 - u_i)) du_i \\
&= 2(1-p) + p \left[\frac{2\sin (2\pi u_i - 2\pi f_i \bmod 1)}{2\pi} \right]_{0}^{1} \\
&= 2(1-p).
\end{align}
Therefore by applying Proposition \ref{prop:hoeff_subgauss_conc} to $\sum_i M_i$, we obtain
\begin{equation} \label{eq:nois_conc_temp1}
\prob(\abs{\sum_i M_i - 2n(1-p)} \geq t) \leq e\cdot\exp\left(-\frac{c^{\prime} t^2}{16n}\right).
\end{equation}
Plugging $t = 2(1-p)n\varepsilon$ in \eqref{eq:nois_conc_temp1} for $\varepsilon \in (0,1)$, we have with probability 
at least $1 - e\cdot\exp\left(-\frac{c^{\prime} (1-p)^2 \varepsilon^2}{4n}\right)$ that the following bound holds.
\begin{equation} \label{eq:nois_conc_temp2}
2(1-p)n(1-\varepsilon) \leq \sum_{i=1}^n M_i \leq 2(1-p)n(1+\varepsilon). 
\end{equation}
Conditioning on the event in \eqref{eq:nois_conc_temp2}, we finally obtain 
from \eqref{eq:nois_conc_temp0} the bound
\begin{align}
\norm{\veczbar - \vechtilbar}_2^2 \ 
\leq 2n - 2(1-p)n(1-\varepsilon) \ 
\leq 2n(p + \varepsilon).
\end{align}
\end{enumerate}
